# Supplementary material for: Measurement Simplification in \rho-POMDP with Performance Guarantees
Source: arXiv:2309.10701 source file (2024-06-17)
Supplement: Supplementary file 1 [file 07-appendix.tex]

\section{APPENDIX}
